# Supplementary material for: Optimal Integrated Task and Path Planning and Its Application to Multi-Robot Pickup and Delivery
Source: arXiv:2403.01277 source file (2024-03-02)
Supplement: Supplementary file 1 [file appendix.tex]

\longversion{
\section*{Appendix}

\subsection{Evaluation of Integrated Planner Complete Results}
\label{appendix_table}
In this section, we have added the complete results we obtained from our experiments for different planners. We have added mean as well as standard deviation as mean(std) in the table. In the tables, $S\%$ denotes success percentages. 
\begin{itemize}
    \item Tables \ref{table:varyW_ITMP_OPT_MS}, \ref{table:varyW_ITMP_OPT_TC}, \ref{table:varyW_ENHSP}, \ref{table:varyW_ENHSP_PRUNED} for various planners for varying workspace 
    \item Tables \ref{table:varyRT_ITMP_OPT_MS}, \ref{table:varyRT_ITMP_OPT_TC}, \ref{table:varyRT_ENHSP}, \ref{table:varyRT_ENHSP_PRUNED}  for various planners for varying RT
    \item Tables  \ref{table:varyRT_COLLAB_ITMP_OPT_MS}, \ref{table:varyRT_COLLAB_ITMP_OPT_TC}, \ref{table:varyRT_COLLAB_ENHSP}, \ref{table:varyRT_COLLAB_ENHSP_PRUNED} for various planners for varying RT with collaboration
\end{itemize}

\setlength{\tabcolsep}{3pt}
%-----------------------------------------------------------------------------------------------
% Varying Workspace size Tables
%-----------------------------------------------------------------------------------------------
\setlength{\tabcolsep}{3pt}
\begin{table}[H]
\caption{Varying workspace size for ITMP with makespan optimization for Figure ~\ref{fig:itmp_varyw}}
\label{table:varyW_ITMP_OPT_MS}
\begin{center}
\begin{tabular}{|c||c||c||c||c|}
\hline
Map Size & S\%  & Time & Makespan & TotalCost \\  \hline \hline
10x10 & 1.0 & 1.8 $\pm$ 0.7 & 30.2 $\pm$ 5.3 & 54.7 $\pm$ 9.9 \\  \hline
20x20 & 1.0 & 2.4 $\pm$ 0.9 & 59.7 $\pm$ 8.6 & 109.0 $\pm$ 19.9 \\ \hline
30x30 & 1.0 & 2.4 $\pm$ 0.6 & 80.8 $\pm$ 18.3 & 145.2 $\pm$ 35.9 \\ \hline
40x40 & 1.0 & 2.7 $\pm$ 1.0 & 115.6 $\pm$ 19.1 & 214.6 $\pm$ 37.8 \\ \hline
50x50 & 1.0 & 2.9 $\pm$ 1.0 & 143.7 $\pm$ 19.0 & 256.1 $\pm$ 50.0 \\ \hline
60x60 & 1.0 & 3.0 $\pm$ 1.1 & 181.4 $\pm$ 26.5 & 333.5 $\pm$ 43.5 \\  \hline
70x70 & 1.0 & 3.4 $\pm$ 1.1 & 197.4 $\pm$ 30.6 & 367.9 $\pm$ 55.8 \\  \hline
80x80 & 1.0 & 3.2 $\pm$ 1.3 & 230.7 $\pm$ 38.5 & 427.7 $\pm$ 69.3 \\  \hline
90x90 & 1.0 & 3.4 $\pm$ 1.1 & 234.4 $\pm$ 40.9 & 433.6 $\pm$ 86.2 \\  \hline
100x100& 1.0 & 3.3 $\pm$ 1.1 & 276.9 $\pm$ 33.2 & 514.2 $\pm$ 78.0 \\  \hline
\end{tabular}
\end{center}
\end{table}

\begin{table}[H]
\caption{Varying workspace size for ITMP with total cost optimization for Figure ~\ref{fig:itmp_varyw}.}
\label{table:varyW_ITMP_OPT_TC} 
\begin{center}
\begin{tabular}{|c||c||c||c||c|}
\hline
Map Size & S\%  & Time & Makespan & TotalCost \\ \hline \hline
10x10 & 1.0 & 4.2 $\pm$ 0.9 & 33.1 $\pm$ 6.0 & 51.3 $\pm$ 8.7  \\ \hline
20x20 & 1.0 & 4.0 $\pm$ 1.8 & 64.7 $\pm$ 10.7 & 100.3 $\pm$ 16.3  \\ \hline
30x30 & 1.0 & 5.0 $\pm$ 1.3 & 84.6 $\pm$ 23.2 & 137.8 $\pm$ 35.0  \\ \hline
40x40 & 1.0 & 5.6 $\pm$ 1.7 & 126.9 $\pm$ 18.1 & 194.1 $\pm$ 38.0  \\ \hline
50x50 & 1.0 & 5.0 $\pm$ 1.5 & 160.0 $\pm$ 30.6 & 240.6 $\pm$ 40.7  \\ \hline
60x60 & 1.0 & 6.0 $\pm$ 2.1 & 196.4 $\pm$ 33.2 & 306.6 $\pm$ 45.6  \\ \hline
70x70 & 1.0 & 5.7 $\pm$ 1.9 & 210.3 $\pm$ 41.2 & 347.8 $\pm$ 53.3  \\ \hline
80x80 & 1.0 & 6.2 $\pm$ 2.5 & 249.1 $\pm$ 43.9 & 393.4 $\pm$ 71.0  \\ \hline
90x90 & 1.0 & 6.2 $\pm$ 2.0 & 252.5 $\pm$ 53.8 & 399.3 $\pm$ 72.3  \\ \hline
100x100& 1.0 & 6.5 $\pm$ 1.5 & 302.9 $\pm$ 58.2 & 473.3 $\pm$ 55.8  \\ \hline
\end{tabular}
\end{center}
\end{table}

\begin{table}[H]
\caption{ Varying workspace size for ENHSP for Figure ~\ref{fig:itmp_varyw}.}
\label{table:varyW_ENHSP}
\begin{center}
\begin{tabular}{|c||c||c||c||c|}
\hline
Map Size & S\%  & Time & Makespan & TotalCost  \\ \hline \hline
10x10 & 0.1 & 3155.6 $\pm$ 1087.9 & 25.3 $\pm$ 3.1 & 41.3 $\pm$ 1.2  \\ \hline
20x20 & 0.0 & 3600.0 $\pm$ 0.0 & nan $\pm$ nan & nan $\pm$ nan  \\ \hline
30x30 & 0.0 & 3600.0 $\pm$ 0.0 & nan $\pm$ nan & nan $\pm$ nan  \\ \hline
40x40 & 0.0 & 3600.0 $\pm$ 0.0 & nan $\pm$ nan & nan $\pm$ nan  \\ \hline
50x50 & 0.0 & 3600.0 $\pm$ 0.0 & nan $\pm$ nan & nan $\pm$ nan  \\ \hline
60x60 & 0.0 & 3600.0 $\pm$ 0.0 & nan $\pm$ nan & nan $\pm$ nan  \\ \hline
70x70 & 0.0 & 3600.0 $\pm$ 0.0 & nan $\pm$ nan & nan $\pm$ nan  \\ \hline
80x80 & 0.0 & 3600.0 $\pm$ 0.0 & nan $\pm$ nan & nan $\pm$ nan  \\ \hline
90x90 & 0.0 & 3600.0 $\pm$ 0.0 & nan $\pm$ nan & nan $\pm$ nan  \\ \hline
100x100& 0.0 & 3600.0 $\pm$ 0.0 & nan $\pm$ nan & nan $\pm$ nan  \\ \hline
\end{tabular}
\end{center}
\end{table}

\begin{table}[H]
\caption{  Varying workspace size for ENHSP Pruned for Figure ~\ref{fig:itmp_varyw}.}
\label{table:varyW_ENHSP_PRUNED}
\begin{center}
\begin{tabular}{|c||c||c||c||c|} 
\hline
Map Size & S\%  & Time & Makespan & TotalCost  \\ \hline \hline
10x10 & 1.0 & 30.6 $\pm$ 29.6 & 40.0 $\pm$ 7.7 & 40.0 $\pm$ 7.7  \\ \hline
20x20 & 0.9 & 1555.3 $\pm$ 1039.4 & 76.7 $\pm$ 9.9 & 76.7 $\pm$ 9.9  \\ \hline
30x30 & 0.0 & 3600.0 $\pm$ 0.0 & nan $\pm$ nan & nan $\pm$ nan  \\ \hline
40x40 & 0.1 & 3432.3 $\pm$ 750.0 & 138.0 $\pm$ nan & 138.0 $\pm$ nan  \\ \hline
50x50 & 0.0 & 3600.0 $\pm$ 0.0 & nan $\pm$ nan & nan $\pm$ nan  \\ \hline
60x60 & 0.0 & 3600.0 $\pm$ 0.0 & nan $\pm$ nan & nan $\pm$ nan  \\ \hline
70x70 & 0.0 & 3600.0 $\pm$ 0.0 & nan $\pm$ nan & nan $\pm$ nan  \\ \hline
80x80 & 0.0 & 3600.0 $\pm$ 0.0 & nan $\pm$ nan & nan $\pm$ nan  \\ \hline
90x90 & 0.0 & 3600.0 $\pm$ 0.0 & nan $\pm$ nan & nan $\pm$ nan  \\ \hline
100x100& 0.0 & 3600.0 $\pm$ 0.0 & nan $\pm$ nan & nan $\pm$ nan  \\ \hline
\end{tabular}
\end{center}
\end{table}

%-----------------------------------------------------------------------------------------------
% Varying Robots and tasks Tables
%-----------------------------------------------------------------------------------------------

\begin{table}[H]
\caption{  Varying Robots (R) and Tasks (T) for ITMP with makespan optimization for Figure ~\ref{fig:itmp_varyrt}.}
\label{table:varyRT_ITMP_OPT_MS}
\begin{center}
\begin{tabular}{|c||c||c||c||c||c|} 
\hline
R & T & S\% & Time & Makespan & TotalCost  \\ \hline %\cline{1-6}
\hline
\multirow[t]{3}{*}{2} & 2 & 1.0 & 0.15 $\pm$ 0.37 & 20.95 $\pm$ 4.7 & 36.7 $\pm$ 8.87  \\ \hline
 & 3 & 1.0 & 1.75 $\pm$ 0.55 & 24.4 $\pm$ 4.66 & 45.0 $\pm$ 9.17  \\ \hline
 & 4 & 1.0 & 2.35 $\pm$ 0.67 & 27.2 $\pm$ 2.38 & 52.6 $\pm$ 4.82  \\ \hline
\hline
\multirow[t]{3}{*}{3} & 3 & 1.0 & 0.25 $\pm$ 0.44 & 21.5 $\pm$ 5.23 & 54.05 $\pm$ 11.19  \\ \hline
 & 4 & 1.0 & 8.8 $\pm$ 3.14 & 23.6 $\pm$ 3.87 & 63.7 $\pm$ 9.89  \\ \hline
 & 5 & 1.0 & 16.95 $\pm$ 6.1 & 25.2 $\pm$ 4.02 & 72.1 $\pm$ 12.89  \\ \hline
\hline
\multirow[t]{3}{*}{4} & 4 & 1.0 & 0.8 $\pm$ 0.41 & 22.25 $\pm$ 4.94 & 73.55 $\pm$ 14.3  \\ \hline
 & 5 & 1.0 & 54.55 $\pm$ 22.8 & 22.7 $\pm$ 3.06 & 80.25 $\pm$ 11.47  \\ \hline
 & 6 & 1.0 & 58.35 $\pm$ 35.44 & 24.6 $\pm$ 2.91 & 89.9 $\pm$ 9.59  \\ \hline
\hline
\multirow[t]{3}{*}{5} & 5 & 1.0 & 1.8 $\pm$ 0.41 & 24.3 $\pm$ 3.39 & 100.2 $\pm$ 11.61  \\ \hline
 & 6 & 1.0 & 546.4 $\pm$ 452.5 & 23.5 $\pm$ 3.24 & 100.1 $\pm$ 16.41  \\ \hline
 & 7 & 0.9 & 391.45 $\pm$ 760.87 & 23.37 $\pm$ 2.83 & 104.89 $\pm$ 13.55  \\ \hline
\hline
\end{tabular}
\end{center}
\end{table}

\begin{table}[H]
\caption{ Varying Robots  (R) and Tasks (T) for ITMP with total cost optimization  for Figure ~\ref{fig:itmp_varyrt}.}
\label{table:varyRT_ITMP_OPT_TC}
\begin{center}
\begin{tabular}{|c||c||c||c||c||c|} 
\hline
R & T & S\% & Time & Makespan & TotalCost  \\ \hline %\cline{1-6}
\hline
\multirow[t]{3}{*}{2} & 2 & 1.0 & 0.1 $\pm$ 0.31 & 21.5 $\pm$ 4.85 & 35.7 $\pm$ 8.37  \\ \hline
 & 3 & 1.0 & 3.45 $\pm$ 0.89 & 26.8 $\pm$ 6.5 & 41.1 $\pm$ 8.14  \\ \hline
 & 4 & 1.0 & 4.95 $\pm$ 1.28 & 28.0 $\pm$ 3.31 & 51.3 $\pm$ 4.78  \\ \hline
\hline
\multirow[t]{3}{*}{3} & 3 & 1.0 & 0.4 $\pm$ 0.5 & 21.9 $\pm$ 5.52 & 51.35 $\pm$ 10.45  \\ \hline
 & 4 & 1.0 & 68.25 $\pm$ 18.36 & 27.1 $\pm$ 2.94 & 49.7 $\pm$ 6.17  \\ \hline
 & 5 & 1.0 & 219.65 $\pm$ 71.18 & 28.8 $\pm$ 5.08 & 63.5 $\pm$ 9.69  \\ \hline
\hline
\multirow[t]{3}{*}{4} & 4 & 1.0 & 1.4 $\pm$ 0.68 & 22.85 $\pm$ 5.08 & 69.3 $\pm$ 11.85  \\ \hline
 & 5 & 1.0 & 2249.7 $\pm$ 570.46 & 27.45 $\pm$ 3.97 & 61.65 $\pm$ 6.08  \\ \hline
 & 6 & 0.0 & 3600.0 $\pm$ 0.0 & nan $\pm$ nan & nan $\pm$ nan  \\ \hline
\hline
\multirow[t]{3}{*}{5} & 5 & 1.0 & 5.25 $\pm$ 1.55 & 25.3 $\pm$ 3.2 & 87.55 $\pm$ 9.57  \\ \hline
 & 6 & 0.0 & 3600.0 $\pm$ 0.0 & nan $\pm$ nan & nan $\pm$ nan  \\ \hline
 & 7 & 0.0 & 3600.0 $\pm$ 0.0 & nan $\pm$ nan & nan $\pm$ nan  \\ \hline
\hline
\end{tabular}
\end{center}
\end{table}

\begin{table}[H]
\caption{ Varying Robots (R) and Tasks (T) for ENHSP  for Figure ~\ref{fig:itmp_varyrt}.}
\label{table:varyRT_ENHSP}
\begin{center}
\begin{tabular}{|c||c||c||c||c||c|} 
\hline
R & T & S\% & Time & Makespan & TotalCost  \\ \hline %\cline{1-6}
\hline
\multirow[t]{3}{*}{2} & 2 & 1.0 & 296.4 $\pm$ 467.0 & 21.55 $\pm$ 4.54 & 37.25 $\pm$ 8.17  \\ \hline
 & 3 & 0.3 & 3311.0 $\pm$ 2851.67 & 25.33 $\pm$ 4.13 & 38.83 $\pm$ 5.74  \\ \hline
 & 4 & 0.0 & 3600.0 $\pm$ 0.0 & nan $\pm$ nan & nan $\pm$ nan  \\ \hline
\hline
\multirow[t]{3}{*}{3} & 3 & 0.1 & 3481.45 $\pm$ 530.17 & 12.0 $\pm$ nan & 28.0 $\pm$ nan  \\ \hline
 & 4 & 0.0 & 3600.0 $\pm$ 0.0 & nan $\pm$ nan & nan $\pm$ nan  \\ \hline
 & 5 & 0.0 & 3600.0 $\pm$ 0.0 & nan $\pm$ nan & nan $\pm$ nan  \\ \hline
\hline
\multirow[t]{3}{*}{4} & 4 & 0.0 & 3600.0 $\pm$ 0.0 & nan $\pm$ nan & nan $\pm$ nan  \\ \hline
 & 5 & 0.0 & 3600.0 $\pm$ 0.0 & nan $\pm$ nan & nan $\pm$ nan  \\ \hline
 & 6 & 0.0 & 3600.0 $\pm$ 0.0 & nan $\pm$ nan & nan $\pm$ nan  \\ \hline
\hline
\multirow[t]{3}{*}{5} & 5 & 0.0 & 3600.0 $\pm$ 0.0 & nan $\pm$ nan & nan $\pm$ nan  \\ \hline
 & 6 & 0.0 & 3600.0 $\pm$ 0.0 & nan $\pm$ nan & nan $\pm$ nan  \\ \hline
 & 7 & 0.0 & 3600.0 $\pm$ 0.0 & nan $\pm$ nan & nan $\pm$ nan  \\ \hline
\hline
\end{tabular}
\end{center}
\end{table}

\begin{table}[H]
\caption{  Varying Robots  (R) and Tasks (T) for ENHSP Pruned  for Figure ~\ref{fig:itmp_varyrt}.}
\label{table:varyRT_ENHSP_PRUNED}
\begin{center}
\begin{tabular}{|c||c||c||c||c||c|} 
\hline
R & T & S\% & Time & Makespan & TotalCost  \\ \hline %\cline{1-6}
\hline
\multirow[t]{3}{*}{2} & 2 & 1.0 & 4.1 $\pm$ 3.97 & 27.3 $\pm$ 4.07 & 27.6 $\pm$ 3.15  \\ \hline
 & 3 & 1.0 & 26.85 $\pm$ 25.42 & 33.7 $\pm$ 3.45 & 34.0 $\pm$ 2.75  \\ \hline
 & 4 & 1.0 & 288.85 $\pm$ 384.8 & 38.9 $\pm$ 3.64 & 39.4 $\pm$ 2.98  \\ \hline
\hline
\multirow[t]{3}{*}{3} & 3 & 0.8 & 1276.5 $\pm$ 1379.28 & 29.88 $\pm$ 4.76 & 31.38 $\pm$ 3.77  \\ \hline
 & 4 & 0.4 & 2561.55 $\pm$ 1316.62 & 36.75 $\pm$ 2.6 & 36.75 $\pm$ 2.6  \\ \hline
 & 5 & 0.0 & 3600.0 $\pm$ 0.0 & nan $\pm$ nan & nan $\pm$ nan  \\ \hline
\hline
\multirow[t]{3}{*}{4} & 4 & 0.0 & 3600.0 $\pm$ 0.0 & nan $\pm$ nan & nan $\pm$ nan  \\ \hline
 & 5 & 0.0 & 3600.0 $\pm$ 0.0 & nan $\pm$ nan & nan $\pm$ nan  \\ \hline
 & 6 & 0.0 & 3600.0 $\pm$ 0.0 & nan $\pm$ nan & nan $\pm$ nan  \\ \hline
\hline
\multirow[t]{3}{*}{5} & 5 & 0.0 & 3600.0 $\pm$ 0.0 & nan $\pm$ nan & nan $\pm$ nan  \\ \hline
 & 6 & 0.0 & 3600.0 $\pm$ 0.0 & nan $\pm$ nan & nan $\pm$ nan  \\ \hline
 & 7 & 0.0 & 3600.0 $\pm$ 0.0 & nan $\pm$ nan & nan $\pm$ nan  \\ \hline
\hline
\end{tabular}
\end{center}
\end{table}

%-----------------------------------------------------------------------------------------------
% Varying robots and task with collaboration Tables
%-----------------------------------------------------------------------------------------------
\begin{table}[H]
\caption{ Varying Robots  (R) and Tasks (T) with varying Z for ITMP with makespan optimization  for Figure ~\ref{fig:itmp_varyrt_collab}.}
\label{table:varyRT_COLLAB_ITMP_OPT_MS}
\begin{center}
\begin{tabular}{|c||c||c||c||c||c|c|} 
\hline
R & T & Z & S\% & Time & Makespan & TotalCost  \\ \hline %\cline{1-6}
\hline
\multirow[t]{3}{*}{2} & \multirow[t]{3}{*}{2} & 4 & 1.0 & 0.1 $\pm$ 0.31 & 20.1 $\pm$ 4.08 & 36.2 $\pm$ 7.9  \\ \hline
 &  & 6 & 1.0 & 1.7 $\pm$ 0.57 & 19.95 $\pm$ 3.93 & 35.5 $\pm$ 7.64  \\ \hline
 &  & 8 & 1.0 & 14.8 $\pm$ 8.1 & 19.95 $\pm$ 3.93 & 36.05 $\pm$ 7.85  \\ \hline
\hline
\multirow[t]{3}{*}{3} & \multirow[t]{3}{*}{3} & 4 & 1.0 & 0.5 $\pm$ 0.51 & 21.6 $\pm$ 3.59 & 56.45 $\pm$ 10.02  \\ \hline
 &  & 6 & 1.0 & 11.05 $\pm$ 3.59 & 21.05 $\pm$ 3.15 & 54.35 $\pm$ 11.6  \\ \hline
 &  & 8 & 1.0 & 833.55 $\pm$ 566.44 & 20.95 $\pm$ 3.15 & 54.65 $\pm$ 10.32  \\ \hline
\hline
\multirow[t]{3}{*}{4} & \multirow[t]{3}{*}{4} & 4 & 1.0 & 1.85 $\pm$ 1.35 & 20.6 $\pm$ 2.85 & 67.8 $\pm$ 10.01  \\ \hline
 &  & 6 & 0.9 & 292.2 $\pm$ 788.63 & 20.0 $\pm$ 2.58 & 65.53 $\pm$ 11.61  \\ \hline
 &  & 8 & 0.2 & 3049.3 $\pm$ 1093.62 & 20.8 $\pm$ 2.28 & 62.8 $\pm$ 9.65  \\ \hline
\hline
\end{tabular}
\end{center}
\end{table}

\begin{table}[H]
\caption{ Varying Robots  (R) and Tasks (T) with varying Z for ITMP with total cost optimization  for Figure ~\ref{fig:itmp_varyrt_collab}.}
\label{table:varyRT_COLLAB_ITMP_OPT_TC}
\begin{center}
\begin{tabular}{|c||c||c||c||c||c|c|} 
\hline
R & T & Z & S\% & Time & Makespan & TotalCost  \\ \hline %\cline{1-6}
\hline
\multirow[t]{3}{*}{2} & \multirow[t]{3}{*}{2} & 4 & 1.0 & 0.2 $\pm$ 0.41 & 20.2 $\pm$ 4.3 & 35.4 $\pm$ 7.54  \\ \hline
 &  & 6 & 1.0 & 1.95 $\pm$ 0.69 & 26.3 $\pm$ 5.28 & 27.2 $\pm$ 3.81  \\ \hline
 &  & 8 & 1.0 & 20.15 $\pm$ 6.89 & 26.3 $\pm$ 5.28 & 27.2 $\pm$ 3.81  \\ \hline
\hline
\multirow[t]{3}{*}{3} & \multirow[t]{3}{*}{3} & 4 & 1.0 & 0.65 $\pm$ 0.49 & 22.3 $\pm$ 4.12 & 52.15 $\pm$ 7.42  \\ \hline
 &  & 6 & 1.0 & 52.2 $\pm$ 23.09 & 26.9 $\pm$ 3.92 & 40.2 $\pm$ 5.02  \\ \hline
 &  & 8 & 0.3 & 2629.2 $\pm$ 1392.11 & 32.0 $\pm$ 3.27 & 32.0 $\pm$ 3.27  \\ \hline
\hline
\multirow[t]{3}{*}{4} & \multirow[t]{3}{*}{4} & 4 & 1.0 & 3.6 $\pm$ 1.5 & 21.35 $\pm$ 3.12 & 60.95 $\pm$ 7.88  \\ \hline
 &  & 6 & 1.0 & 1086.45 $\pm$ 413.77 & 24.95 $\pm$ 3.2 & 45.2 $\pm$ 5.22  \\ \hline
 &  & 8 & 0.0 & 3600.0 $\pm$ 0.0 & nan $\pm$ nan & nan $\pm$ nan  \\ \hline
\hline
\end{tabular}
\end{center}
\end{table}

\begin{table}[H]
\caption{Varying Robots  (R) and Tasks (T) with collaboration for ENHSP  for Figure ~\ref{fig:itmp_varyrt_collab}.}
\label{table:varyRT_COLLAB_ENHSP}
\begin{center}
\begin{tabular}{|c||c||c||c||c||c|} 
\hline
R & T & S\% & Time & Makespan & TotalCost  \\ \hline %\cline{1-6}
\hline
2 & 2 & 1.0 & 65.5 $\pm$ 98.21 & 26.3 $\pm$ 5.28 & 27.2 $\pm$ 3.81  \\ \hline
3 & 3 & 0.0 & 3600.0 $\pm$ 0.0 & nan $\pm$ nan & nan $\pm$ nan  \\ \hline
4 & 4 & 0.0 & 3600.0 $\pm$ 0.0 & nan $\pm$ nan & nan $\pm$ nan  \\ \hline

\hline
\end{tabular}
\end{center}
\end{table}

\begin{table}[H]
\caption{Varying Robots  (R) and Tasks (T) for ENHSP Pruned  for Figure ~\ref{fig:itmp_varyrt_collab}.}
\label{table:varyRT_COLLAB_ENHSP_PRUNED}
\begin{center}
\begin{tabular}{|c||c||c||c||c||c|}
\hline
R & T & S\% & Time & Makespan & TotalCost  \\ \hline 
\hline
2 & 2 & 1.0 & 5.85 $\pm$ 6.76 & 26.3 $\pm$ 5.28 & 27.2 $\pm$ 3.81  \\ \hline
3 & 3 & 0.7 & 1797.45 $\pm$ 1443.77 & 31.29 $\pm$ 2.79 & 31.29 $\pm$ 2.79  \\ \hline
4 & 4 & 0.0 & 3600.0 $\pm$ 0.0 & nan $\pm$ nan & nan $\pm$ nan  \\ \hline

\hline
\end{tabular}
\end{center}
\end{table}

}
